# Supplementary material for: Bridging-induced Aggregation in Neutral Polymers: Dynamics and Morphologies
Source: arXiv:2504.00703 ancillary file (2025-04-01)
Supplement: Supplementary file 1 [file Supp.pdf]

## Supporting Information

### **Bridging-induced Aggregation in Neutral Polymers: Dynamics and Morphologies**

Hitesh Garg<sup>1, 2, a)</sup> and Satyavani Vemparala<sup>1, 2, b)</sup>

<sup>1)</sup>*The Institute of Mathematical Sciences, C.I.T. Campus, Taramani,  
Chennai 600113, India*

<sup>2)</sup>*Homi Bhabha National Institute, Training School Complex, Anushakti Nagar,  
Mumbai, 400094, India*

---

<sup>a)</sup>Electronic mail: [hiteshgarg@imsc.res.in](mailto:hiteshgarg@imsc.res.in)

<sup>b)</sup>Electronic mail: [vani@imsc.res.in](mailto:vani@imsc.res.in)

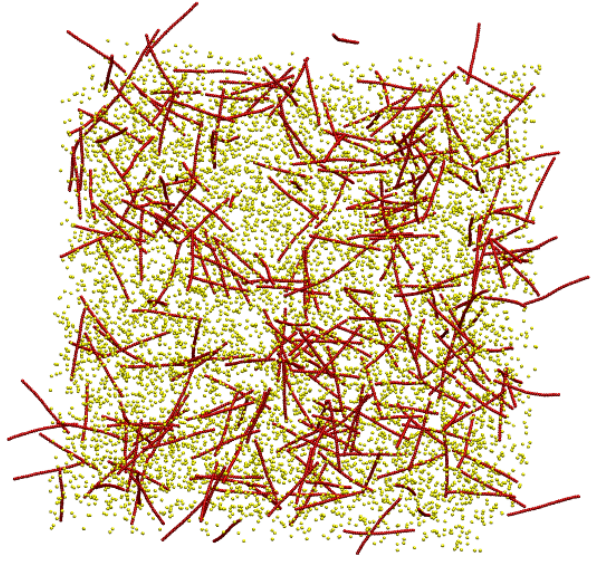

FIG. S1. The *WCA* interaction between all the particles are unable to induce aggregation. The density of crowders is low to induce aggregation due to depletion effect.

TABLE S1. The critical values of transition  $\epsilon_{mc}^*$  for different value of crowder number densities.

| <i>density</i>        | <i>rigid</i> | <i>flexible</i> | <i>single chain</i> |
|-----------------------|--------------|-----------------|---------------------|
| $9 \times 10^{-3}$    | 1.3          | 1.2             | 1.25                |
| $2.66 \times 10^{-3}$ | 1.7          | 1.4             | 1.45                |
| $1.12 \times 10^{-3}$ | 2.0          | 1.7             | 1.59                |
| $5.76 \times 10^{-4}$ | 2.3          | 1.9             | 1.72                |
| $3.33 \times 10^{-4}$ | 2.6          | 2.1             | 1.90                |

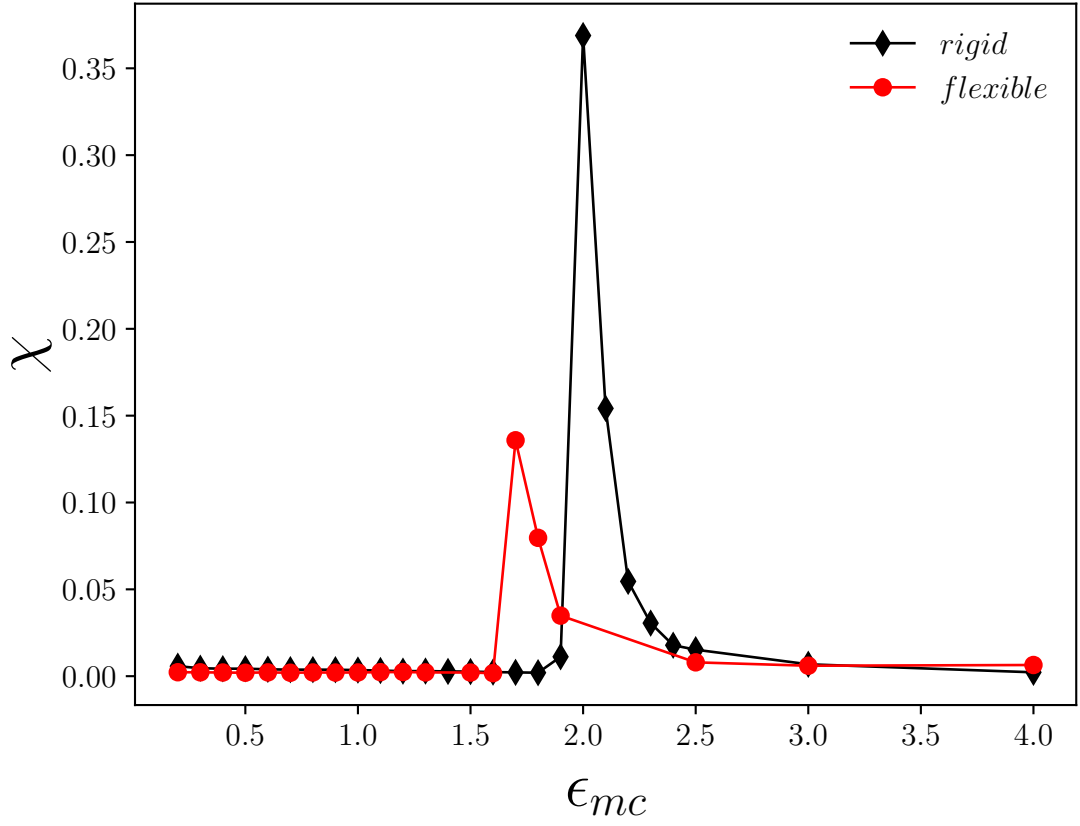

FIG. S2. Relative fluctuation ( $\chi$ ) in the pair energy per particle as a function of the monomer-crowder interaction strength ( $\epsilon_{mc}$ ) for rigid and flexible polymer chains. The critical aggregation thresholds are identified at  $\epsilon_{mc}^* = 2.0$  for rigid chains and  $\epsilon_{mc}^* = 1.7$  for flexible chains.

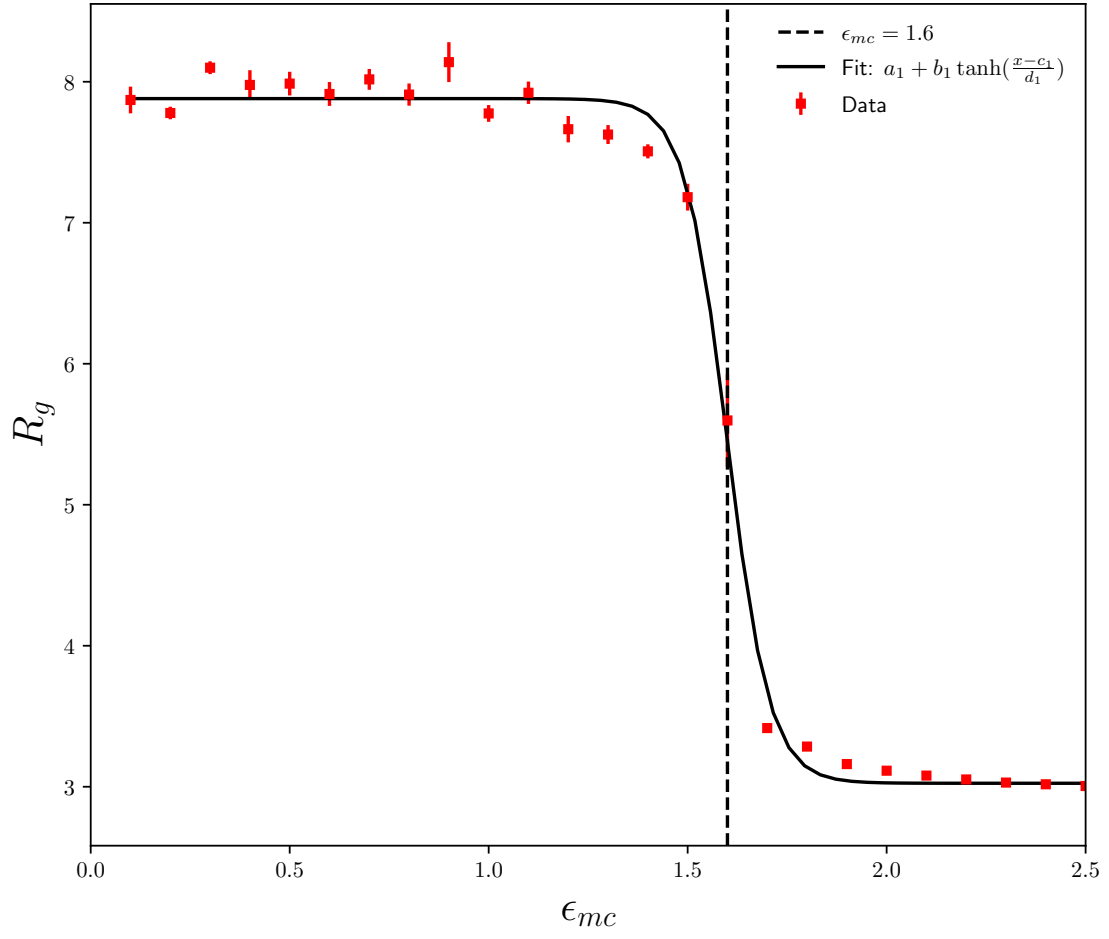

FIG. S3. The variation of radius of gyration with  $\epsilon_{mc}$ . The monomer-monomer has WCA interaction

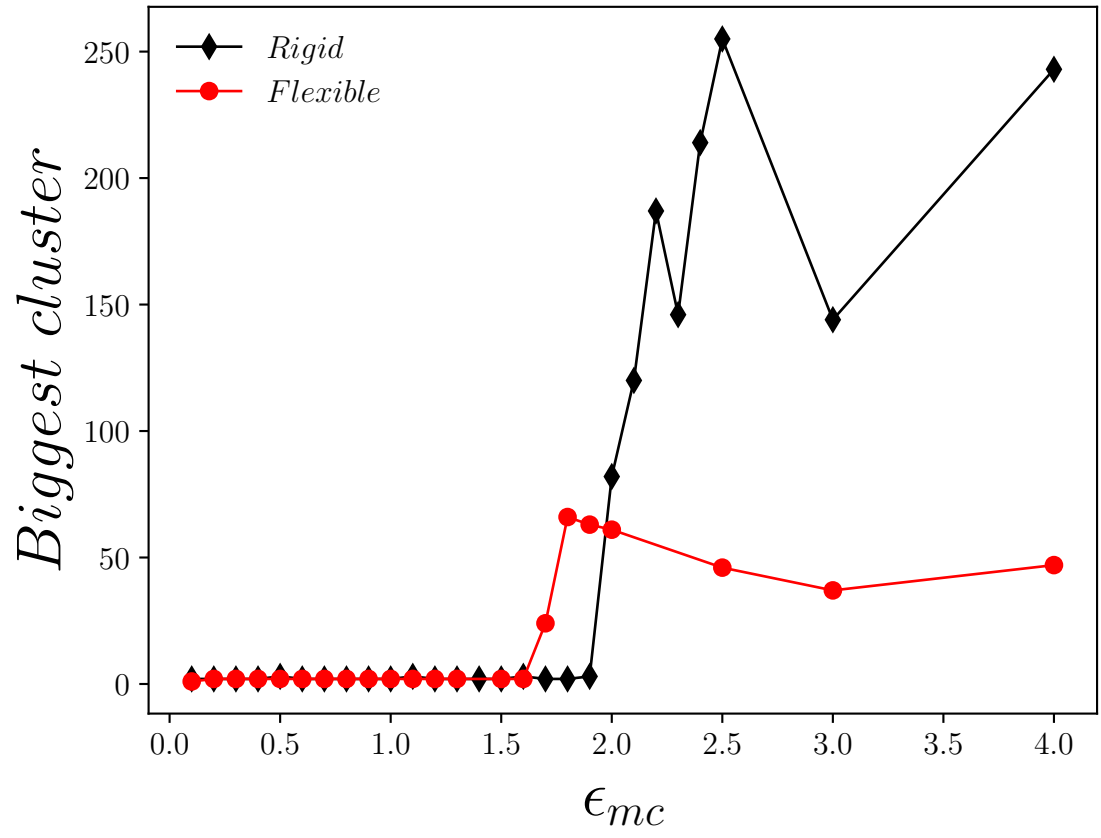

FIG. S4. The variation of the biggest cluster size with  $\epsilon_{mc}$  for rigid rod and flexible chains

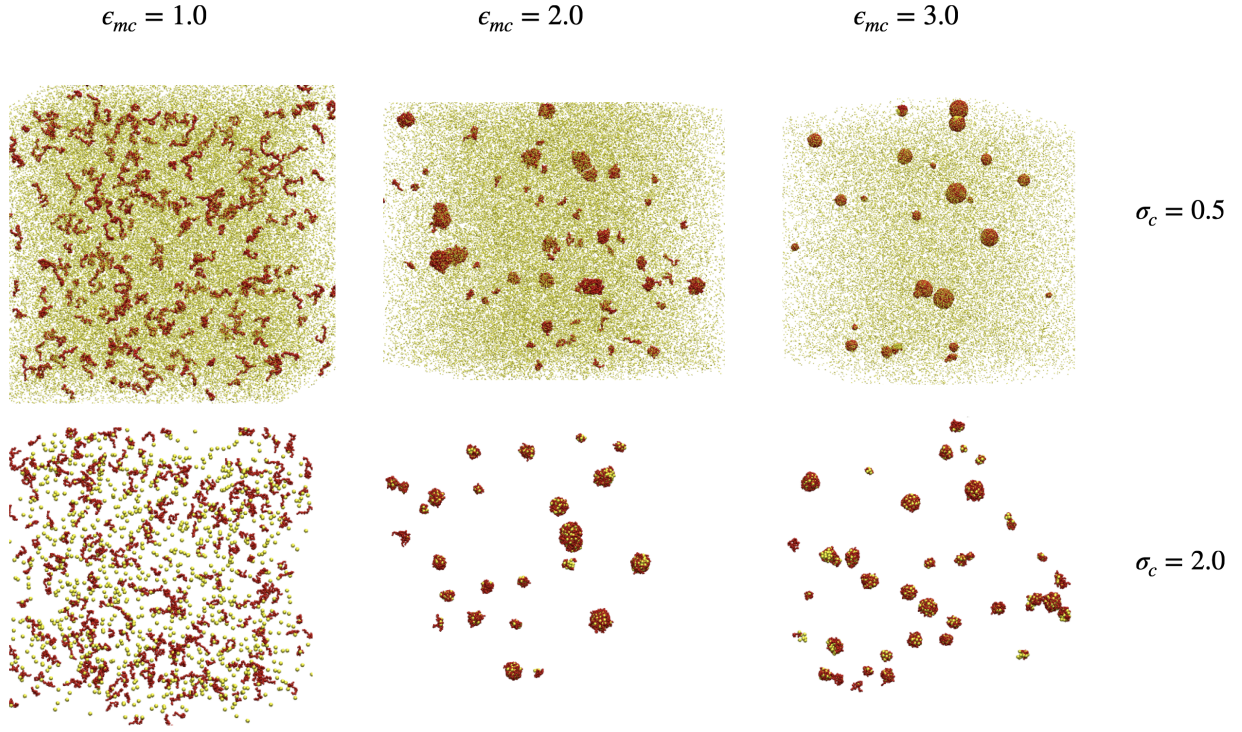

FIG. S5. The snapshots of polymers at different monomer-crowder attraction  $\epsilon_{mc}$  for flexible chains for two different crowder sizes.

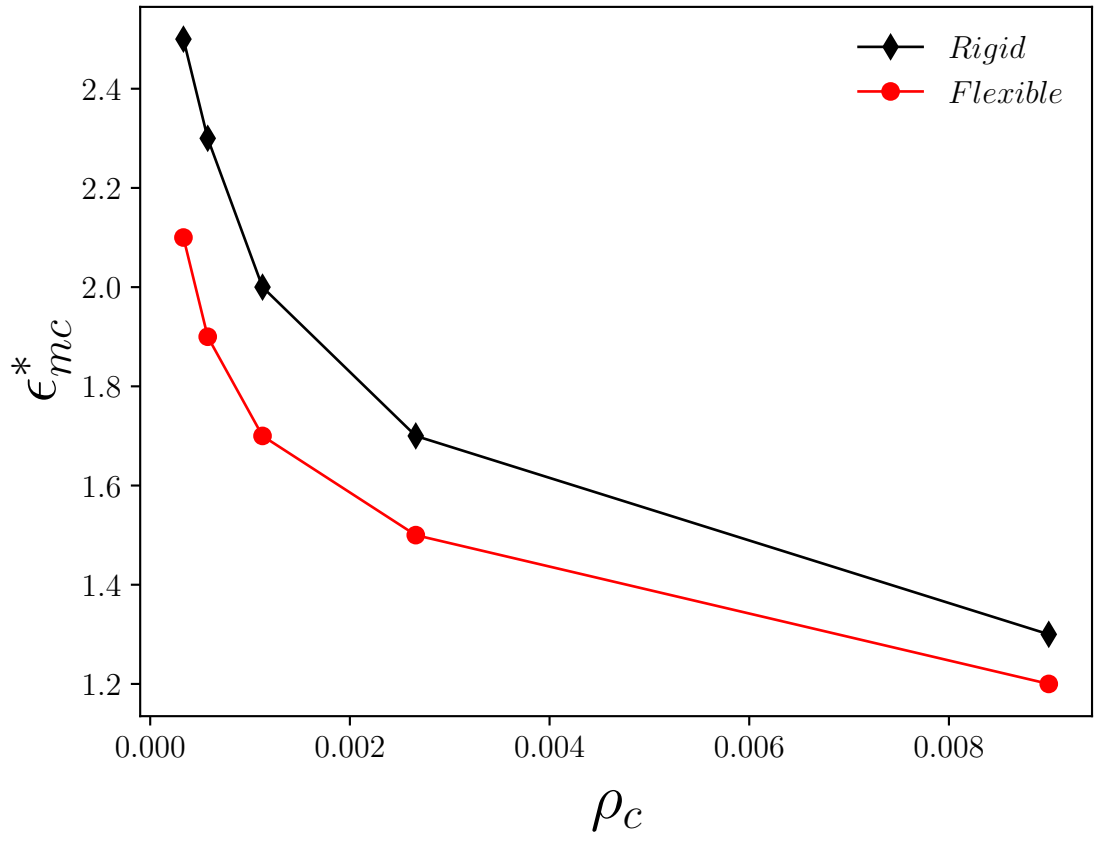

FIG. S6. The variation of critical value of transition  $\epsilon_{mc}^*$  with number density of crowders. It increases linearly with box size.

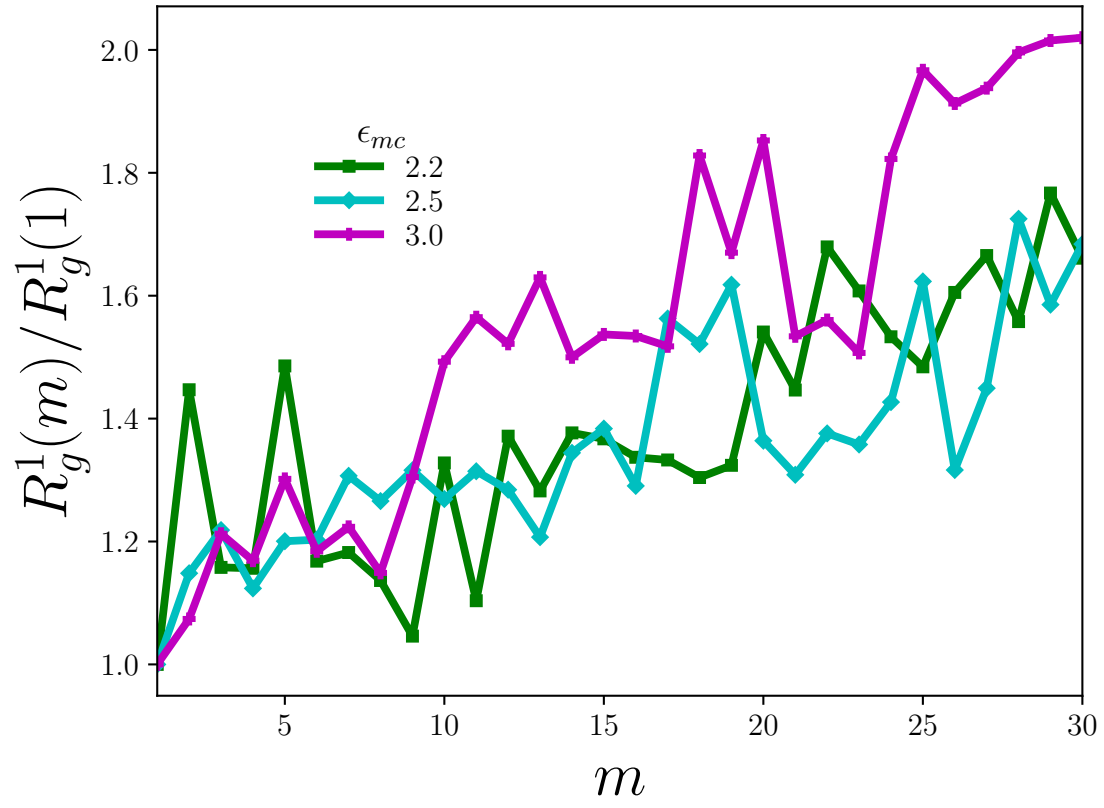

FIG. S7. Scaled radius of gyration of a single flexible chain belonging to an aggregate of size  $m$ , as a function of  $m$  for different  $\epsilon_{mc}$ .
